# Supplementary material for: HalluPrism: When Multimodal Uncertainty Should Diagnose, Not Decide
Source: arXiv:2608.29193 source file (2026-08-29)
Supplement: Supplementary file 1 [file Perturbation-Probes.tex]

\subsection{Perturbation Probes}
\label{subsec:perturbation_probes}

We measure how the same prediction behaves when pressure is placed on different parts of the input. The clean answer $\hat{y}$ is the baseline. Each probe produces a perturbed answer $\tilde{y}$. We compare $\hat{y}$ and $\tilde{y}$ using answer change and confidence change. Let $\mathrm{flip}(\hat{y},\tilde{y})=1$ if the perturbed answer differs from the clean answer after normalization, and $0$ otherwise. Let $\Delta c(\hat{y},\tilde{y})=|c(\hat{y})-c(\tilde{y})|$. Flips capture discrete instability, while confidence shifts capture softer changes when the answer remains unchanged.

The \textbf{visual score} $V$ measures sensitivity to degraded visual evidence. In the cone-car example, this tests whether the answer changes when the cone is blurred, cropped, darkened, or corrupted by noise. We construct $K=4$ image variants while keeping the prompt fixed: Gaussian blur, center crop, brightness reduction, and Gaussian noise. For the $k$-th perturbed answer $\tilde{y}^{v}_{k}$, we define:
\begin{equation}
\begin{split}
& V =
0.6\cdot\frac{1}{K}
\sum_{k=1}^{K}
\mathrm{flip}(\hat{y},\tilde{y}^{v}_{k})
\\
& \qquad
+0.4\cdot
\min\left(
2\cdot\frac{1}{K}
\sum_{k=1}^{K}
\Delta c(\hat{y},\tilde{y}^{v}_{k}),
1
\right).
\end{split}
\label{eq:visual_score}
\end{equation}
The larger flip weight makes changed answers the primary signal of visual fragility.

The \textbf{language-prior score} $L$ measures answer survival when visual evidence is removed. In the cone-car example, this tests whether the model still gives the same left-right answer after both objects are removed by replacing the image with a blank canvas. We replace the image with a uniform blank image $I_{\mathrm{blank}}$ and keep the same prompt. Let $\tilde{y}^{\ell}$ be the blank-image answer. We define:
\begin{equation}
\begin{split}
& L =
\mathbf{1}[\mathrm{match}(\hat{y},\tilde{y}^{\ell})]
\cdot
\min\left(
\frac{c(\tilde{y}^{\ell})}{c(\hat{y})+\epsilon},
1
\right).
\end{split}
\label{eq:language_score}
\end{equation}
A high $L$ means that the same answer persists with similar confidence without the original image. It is a behavioral marker. It does not imply that the model ignores the image in every case.

The \textbf{alignment score} $A$ measures sensitivity to cross-modal binding pressure. It tests whether the answer remains stable when the relevant image-text relation is re-queried or swapped. We use a grounding probe for all datasets and add a relation-swap probe when the task has an explicit perturbable relation. Visual Spatial Reasoning (VSR) is the clearest case, because its prompts contain spatial relations such as \textit{left}, \textit{right}, \textit{above}, \textit{below}, \textit{in front of}, and \textit{behind}. In the cone-car example, if the clean prompt asks whether the cone is to the left of the car, the relation-swapped prompt asks the corresponding right-of question. A relation-sensitive model should not preserve the same normalized answer under both prompts. Let $\tilde{y}^{a}_{\mathrm{ground}}$ be the grounding-prompt answer, and let $\tilde{y}^{a}_{\mathrm{rel}}$ be the relation-swapped answer when such a swap is available. We define:
\begin{equation}
\begin{split}
& P_g =
0.5\cdot
\mathrm{flip}(\hat{y},\tilde{y}^{a}_{\mathrm{ground}})
+
\min(
\Delta c(\hat{y},\tilde{y}^{a}_{\mathrm{ground}}),
0.5
),
\\
& P_r =
\mathbf{1}[\mathrm{available}]
\cdot
\mathbf{1}[
\mathrm{norm}(\tilde{y}^{a}_{\mathrm{rel}})
=
\mathrm{norm}(\hat{y})
],
\\
& A =
\begin{cases}
\min(0.4P_g+0.6P_r,1), & \mathrm{if\ available},\\
\min(P_g,1), & \mathrm{otherwise}.
\end{cases}
\end{split}
\label{eq:alignment_score}
\end{equation}
The relation term receives larger weight when available because it directly tests whether the model preserves the same answer under a controlled relation swap where the expected answer should change.
