# Supplementary material for: HalluPrism: When Multimodal Uncertainty Should Diagnose, Not Decide
Source: arXiv:2608.29193 source file (2026-08-29)
Supplement: Supplementary file 2 [file Responsible-NLP-Checklist.tex]

\section{Responsible NLP Checklist}
\label{app:responsible_nlp_checklist}

We answer the Responsible NLP Checklist following the ACL Rolling Review (ARR) format. For each item, we provide a direct answer and point to the relevant part of the paper or appendix. When an item is not applicable, we state why. The checklist is intended to clarify ethical, reproducibility, artifact, annotation, and computational details for reviewers.

\begin{table*}[t]
\centering
\scalebox{0.78}{
\begin{tabular}{p{0.07\linewidth}p{0.08\linewidth}p{0.50\linewidth}p{0.24\linewidth}}
\toprule
\textbf{Item} & \textbf{Answer} & \textbf{Response} & \textbf{Where Addressed} \\
\midrule
A1 & Yes & We describe limitations of the behavioral source-signature interpretation, dataset scope, computational overhead, and conditional nature of routing. & Limitations; Appendix~\ref{app:ethics_responsible_use} \\
A2 & Yes & We discuss risks from over-trusting source scores, treating them as causal explanations, using them as safety certificates, and applying routing in high-stakes settings without validation. & Limitations; Appendix~\ref{app:ethics_responsible_use} \\
A3 & Yes & The abstract and introduction state the main claim: diagnosis should be central to multimodal uncertainty, and \HalluPrism{} measures visual fragility, language-prior reliance, and cross-modal alignment instability. & Abstract; Section~1 \\
A4 & Yes & We used AI writing assistance for language editing, LaTeX drafting, and checklist preparation. The authors verified all claims, citations, mathematical statements, experiments, and final wording. & Checklist disclosure \\
\midrule
B & Yes & We use public datasets, public model artifacts, and derived evaluation artifacts. We document their use, access conditions, and release boundaries. & Appendix~\ref{app:artifact_license_data_statement} \\
B1 & Yes & We cite the creators of all datasets, models, and relevant software artifacts used in the paper. & References; Section~4; Appendix~\ref{app:artifact_license_data_statement} \\
B2 & Yes & We report license and access notes for HallusionBench, POPE, VSR, VizWiz-VQA, Gemma 4, Qwen3-VL, LLaVA-Mistral, and LLaVA-Vicuna. & Appendix~\ref{app:artifact_license_data_statement} \\
B3 & Yes & We use all artifacts for research evaluation, model analysis, and diagnostic benchmarking. We do not redistribute model weights or raw images when the original access terms restrict redistribution. & Appendix~\ref{app:artifact_license_data_statement} \\
B4 & Yes & We discuss data sensitivity, especially for VizWiz-VQA, where images and questions may come from blind or low-vision users and may contain private environments or personal objects. & Appendix~\ref{app:artifact_license_data_statement}; Appendix~\ref{app:ethics_responsible_use} \\
B5 & Yes & We document dataset coverage, task stress factors, failure-family mappings, and benchmark roles. & Table~1; Appendix~\ref{app:additional_results}; Appendix~\ref{app:artifact_license_data_statement} \\
B6 & Yes & We report dataset sizes, pooled model-output counts, failure-family counts, and per-dataset evaluation roles. & Table~1; Appendix~\ref{app:additional_results} \\
\midrule
C & Yes & We run computational experiments using open-weight or publicly accessible MLLMs under deterministic decoding. & Section~4; Appendix~\ref{app:compute} \\
C1 & Partial & We report the number of evaluated model-output instances, number of forward passes, inference-only nature of the experiments, and a hardware-reporting table. Final GPU type, wall-clock time, and GPU-hours should be filled from the execution logs before submission. & Appendix~\ref{app:compute} \\
C2 & Yes & We describe deterministic decoding, response length, classifiers, cross-validation, scalarization rules, routing policies, and prompt templates. & Section~3; Section~4; Appendix~\ref{app:prompt_catalog}; Appendix~\ref{app:compute} \\
C3 & Yes & We report summary statistics, full source profiles, pass counts, diagnosis results with fold variability where applicable, risk-coverage values, and routing fix/break rates. & Section~5; Appendix~\ref{app:additional_results} \\
C4 & Yes & We report prompt templates, perturbation parameters, answer normalization rules, image-enhancement parameters, scalarization formulas, and classifier families. & Section~3; Appendix~\ref{app:prompt_catalog}; Appendix~\ref{app:compute} \\
\midrule
D & Partial & The main experiments do not collect new human-subject data. We include a human-audit protocol as an optional semantic plausibility check. If completed, the final version should report recruitment, compensation, agreement, adjudication, and approval or exemption status. & Appendix~\ref{app:human_audit} \\
D1 & Yes & We provide the full audit instructions shown to annotators. & Appendix~\ref{app:human_audit} \\
D2 & To Fill & The current draft specifies the audit design, but final recruitment platform, annotator pool, and compensation details must be added if the audit is completed. & Appendix~\ref{app:human_audit} \\
D3 & N/A & We do not collect new user data for the main experiments. We use public benchmarks. If a human audit is completed, annotators label benchmark examples rather than providing personal data. & Appendix~\ref{app:artifact_license_data_statement}; Appendix~\ref{app:human_audit} \\
D4 & To Fill & The main benchmark-only experiments do not require new human-subject data collection. If the human audit is completed, the final paper should report ethics-board approval, exemption, or institutional determination. & Appendix~\ref{app:human_audit} \\
D5 & To Fill & If the human audit is completed, the final paper should report the basic demographic and geographic characteristics collected for annotators, subject to privacy and institutional rules. & Appendix~\ref{app:human_audit} \\
\bottomrule
\end{tabular}
}
\caption{Responsible NLP Checklist responses for \HalluPrism{}. We use ``N/A'' only when the item does not apply to the submitted work.}
\label{tab:responsible_nlp_checklist_overview}
\end{table*}

\subsection{A. For Every Submission}
\label{app:checklist_every_submission}

\paragraph{A1. Did we describe the limitations of the work?}
Yes. We discuss limitations in the main paper and in Appendix~\ref{app:ethics_responsible_use}. \HalluPrism{} is a behavioral diagnostic layer, not a causal explanation of hidden mechanisms inside an MLLM. The source scores depend on the probe family and should be read as a perturbation-response signature rather than independent ground-truth causes. We also state that the evaluation does not cover video, multi-image reasoning, medical, document-heavy expert settings, or latency-critical deployment.

\paragraph{A2. Did we discuss potential risks of the work?}
Yes. We discuss risks in Appendix~\ref{app:ethics_responsible_use}. The main risks are (i) over-trusting the source signature as a complete safety certificate, (ii) treating behavioral scores as causal explanations, (iii) applying correction prompts in settings where they may break correct answers, and (iv) using the method in high-stakes settings without domain-specific validation and human oversight.

\paragraph{A3. Do the abstract and introduction summarize the paper's main claims?}
Yes. The abstract and introduction state the diagnosis-first claim, define \HalluPrism{}, describe the three source scores $(V,L,A)$, and summarize the empirical patterns. They also state that source signatures are diagnostic and routing objects, not scalar abstention replacements.

\paragraph{A4. Did we use AI writing assistants when working on the paper?}
Yes. AI writing assistance was used for language editing and polishing LaTeX tables. The authors verified the scientific claims, citations, experimental results, mathematical statements, and final text. AI assistance was not treated as authorship.

\subsection{B. Scientific Artifacts}
\label{app:checklist_scientific_artifacts}

\paragraph{B. Did we use or create scientific artifacts?}
Yes. We use public benchmark datasets, public model artifacts, and derived evaluation artifacts. We document these in Appendix~\ref{app:artifact_license_data_statement}.

\paragraph{B1. Did we cite the creators of artifacts used in the paper?}
Yes. We cite the original creators of HallusionBench, POPE, VSR, VizWiz-VQA, Gemma 4, Qwen3-VL, LLaVA-Mistral, and LLaVA-Vicuna in the main bibliography. Dataset and model roles are summarized in Section~4 and Appendix~\ref{app:artifact_license_data_statement}.

\paragraph{B2. Did we discuss artifact licenses or terms of use?}
Yes. Appendix~\ref{app:artifact_license_data_statement} reports license or access notes for each dataset and model artifact. We do not redistribute raw benchmark images or model weights. We release only scripts, prompts, derived metadata, normalized predictions, source scores, and aggregate tables when permitted by the original artifact terms.

\paragraph{B3. Did we discuss consistency with intended use?}
Yes. We use all artifacts for research evaluation, model analysis, and diagnostic benchmarking. We do not use the datasets to train a deployed model, infer private attributes, identify individuals, or make decisions about real users. For derived artifacts, we specify that release should remain compatible with the original dataset and model access terms.

\paragraph{B4. Did we discuss personally identifying information or offensive content?}
Yes. Appendix~\ref{app:artifact_license_data_statement} and Appendix~\ref{app:ethics_responsible_use} discuss the sensitivity of visual datasets. VizWiz-VQA is especially relevant because it contains images and questions from blind or low-vision users. We do not redistribute raw images, and we recommend that downstream users inspect dataset privacy notes and licenses before reusing visual content.

\paragraph{B5. Did we provide artifact documentation?}
Yes. Table~1 and Appendix~\ref{app:artifact_license_data_statement} document each benchmark's role in the evaluation. Appendix~\ref{app:additional_results} gives dataset composition, failure-family coverage, source-profile statistics, and fixed-dataset diagnostic controls.

\paragraph{B6. Did we report relevant dataset statistics?}
Yes. Table~1 reports the main evaluation suite. Appendix~\ref{app:additional_results} reports per-dataset counts, pooled counts, failure-family counts, and model-output counts. We evaluate $58{,}440$ model-dataset outputs across four benchmarks and four model families.

\subsection{C. Computational Experiments}
\label{app:checklist_computational_experiments}

\paragraph{C. Did we run computational experiments?}
Yes. We run deterministic inference experiments with four MLLM families over four multimodal benchmarks. We do not fine-tune the evaluated MLLMs.

\paragraph{C1. Did we report model parameters, computational budget, and infrastructure?}
Partially. We report the inference-only design, number of evaluated examples, number of forward passes, and the approximate full diagnosis-plus-routing pass budget in Appendix~\ref{app:compute}. We also provide a hardware-reporting table. The final version should fill GPU type, number of GPUs, wall-clock runtime, and GPU-hours from the execution logs. If exact energy measurements are unavailable, we report forward-pass counts and deterministic decoding settings rather than inventing carbon estimates.

\paragraph{C2. Did we discuss the experimental setup and hyperparameters?}
Yes. Section~4 describes datasets, model families, decoding settings, and classifier families. Appendix~\ref{app:prompt_catalog} reports base prompts, diagnostic probe prompts, perturbation settings, generic intervention, matched interventions, and answer-normalization rules. Section~3 gives the formulas for source signatures, scalarization, and routing metrics.

\paragraph{C3. Did we report descriptive statistics about results?}
Yes. Section~5 reports source-profile summaries, diagnosis AUROC, feature importance, abstention AUROC, and routing accuracy, fix rate, and break rate. Appendix~\ref{app:additional_results} reports full model-dataset source profiles, intervention deltas, diagnosis tables, dataset-identity controls, within-dataset controls, risk-coverage values, and routing win counts.

\paragraph{C4. Did we report implementation and parameter settings for packages or preprocessing?}
Yes. We report image perturbation parameters, answer normalization, scalarization formulas, routing prompts, and intervention parameters in Section~3 and Appendix~\ref{app:prompt_catalog}. We also report the classifier families used for diagnosis: logistic regression, XGBoost, and LightGBM.

\subsection{D. Human Annotation Or Human Participants}
\label{app:checklist_human_participants}

\paragraph{D. Did we use human annotators or human participants?}
Partially. The main experiments do not collect new human-subject data. We include a human-audit protocol as a semantic plausibility check for source labels. If the audit is completed, the final submission should report recruitment, compensation, agreement, adjudication, and ethics-board approval or exemption.

\paragraph{D1. Did we report the full text of instructions given to participants?}
Yes, for the planned audit protocol. Appendix~\ref{app:human_audit} provides the full annotation instructions, label rubric, visible and hidden fields, and adjudication procedure.

\paragraph{D2. Did we report recruitment and payment information?}
To be filled if the audit is completed. The current protocol defines the annotation task and reporting fields. The final version should specify the recruitment source, annotator qualification criteria, compensation rate, estimated annotation time, and why the payment is adequate.

\paragraph{D3. Did we discuss whether and how consent was obtained from people whose data is used or curated?}
Not applicable to the main experiments. We use public benchmark datasets and do not collect new user images. If the human audit is completed, annotators should provide informed consent according to the institutional or platform-specific annotation protocol.

\paragraph{D4. Was the data collection protocol approved or determined exempt by an ethics review board?}
To be filled if the audit is completed. The benchmark-only experiments do not create new human-subject data. If the audit is run with human annotators, the final paper should report whether the protocol was approved, determined exempt, or not considered human-subjects research under the relevant institutional policy.

\paragraph{D5. Did we report demographic and geographic characteristics of annotators?}
To be filled if the audit is completed. The final paper should report the demographic and geographic characteristics collected under the annotation protocol, subject to privacy constraints. If these characteristics are not collected, the paper should state that explicitly and justify the choice.

\subsection{Checklist Completion Note}
\label{app:checklist_completion_note}

This checklist should be synchronized with the ARR/OpenReview submission form before final submission. Items marked \textit{To Fill} should not remain unresolved in the submitted version if the human audit is included as a completed result. If the audit is not completed, the paper should keep it as a protocol-only appendix or remove audit-result tables and state that larger human validation remains future work.
